# Supplementary material for: 3D-IntPhys: Towards More Generalized 3D-grounded Visual Intuitive Physics under Challenging Scenes
Source: arXiv:2304.11470 source file (2023-04-22)
Supplement: Supplementary file 1 [file supp_old.tex]

%%%%%%%%%%%%%%%%%%%%%%%%%%%%%%%%%%%%%%%%%%%%%%%%%%%%%%%%%%%%


\appendix

\section{3D point representation from trained pixelNerf}\label{sup-3d-represnetation}

 For a dataset that contains $N_t$ trajectory videos, each video  has $N_f$ frames and each frame is taken from $N_v$ views. Actually we have $N_t * N_f * N_v$ images from $N_{s} = N_t * N_f$ different scenes. We note $\textbf{I}^{(i, j, k)}$ as the image from $i$-th trajectory, $j$-th frame and $k$-th view. We can train a pixelNeRF $F_{\phi}$ on the a subset of the trajectories and it can generalize in other trajectories.

Then for scene $s \in \{1, 2, ..., N_s\}$ with $O_s$ target object(such as fluid, cube), we sample a volumetric space $\textbf{R}(T)$ sized $T * T * T$ in the middle of the desk which can cover the scene and query all the $T^3$ points in the volume to get $(\textbf{c}, \sigma) = F_{\phi}(\textbf{R}(T))$. Then we can select from the $\textbf{R}(T)$ using the density value $\sigma$ to get the point cloud of objects in the scene(container, water, box, robot arm, table): $\textbf{R}_{obj}(T) = \{t \in \textbf{R}(T) | \sigma(t) > \sigma_{min}\}$, where $\sigma_{min}$ is the lowest bar for object density. Here we use color as prior information to segment out the points we want to modeling(water, box). Specifically, for target points which forms a object $o_{i} \in \{1, 2, 3, ..., O_s\}$, we can get the point cloud of this object: $\textbf{R}_{o_{i}}(T) =  \{t \in \textbf{R}_{obj}(T) | \textbf{c}(t) \in r(o_i)\}$ where $r(o_i)$ is the color set for object $o_i$. We note the final point cloud of scene $s$ as $p_{s} = \{p_{s}^{1}, p_{s}^{2}, ..., p_{s}^{O_s}\}$.

Then we can do sparse sampling of each point cloud using FPS (Farthest Point Sampling), which can sample small subset of the target point cloud and maintain the shape of it. To facilitate the learning of particle-based dynamics, we set the size after sampling fixed.


\section{Graph-Based Dynamics Model without Particle-level Correspondence} \label{dpi-wo-correspondece}

As we described in Section 3.2 in the paper, the attributes $a^{v}_{i}$ of a vertex $v_i$ in the built graph includes: 1. velocity of this point in the past frames, 2. attributes of the point (rigid, fluid, granular). To get the velocity of $v$, we should have the history position of $v$. However, since the point-cloud is directly generated from images and do not have particle-level labels. It is hard to get the velocity of one specific points in the graph, since we lack one-to-one correspondence between points. To deal with this problem and make us able to learn complex fluid dynamics without particle-level correspondence, we make small modifications on the original graph-based model in \cite{DPI}.

We assume that we know the dense-labeled states of some known fully-actuated shape like desk and cups that is connected to the robot arms. Here we will list one specific scenario where a cup of water is poured out into another cup. In this case, we have two different types of points: points for fluid and points for cups, we name the states of them in time step $t$ as $V_{P}^{t}=\{v_{P, i}^{t}\}$ and $V_{S}^{t}=\{v_{S, i}^{t}\}$ respectively. For the particle encoder $Q_v$, if the particle belongs to the cups, then the input of particle encoder contains  $n_s$ history states before $t_0$ : $\{V_{S}^{(t_0-n_s):t_0}\}$. If the particle belongs to the water, then we have no history states, so the input of $Q_v$ is all-zero. 


By adding the relative position between receiver and sender points, we can pass the momentum of $V_P$ to $V_S$. Compared with human intuition, we can get an intuitive prediction of the movement of water by simply knowing the past movement of the cup without knowing the past movement of water.




It should also be noted that all the inputs of the dynamics predictor are actually velocity of points or relative position instead of raw position. We do this to make the model translation-invariant so it can be much more generalized when we translate the raw scenario into different scale of coordinate. 



% \section{Online Rolling}

% Online rolling prediction is one of the most significant m


\section{Model Structure of 3D-IntPhys}

Our 3D-IntPhys model can be divided into two parts : one for visual perception, the other for dynamics prediction.

\paragraph{Conditional NeRF} The structure follows that in\cite{pixelnerf}. For the feature encoder in conditional NeRF,  We employ a ResNet34 backbone to extract  feature pyramid by using the feature map prior to the first pooling layer and after the first ResNet 3 layers. Before the training starts, we initialize the weight of feature extractor of the scene using ImageNet pretrained weight. For the NeRF function $f$, We use  fully-connected ResNet
architecture with 5 ResNet blocks with width 512. 

\paragraph{Dynamics Predictor} We use 3-Layer DNN activated by ReLu function with hidden unit sized $150$ for Encoder of both edge and vertex: $Q_e$ and $Q_v$, the propagators $P_e$ and $P_v$ are 1-Layer linear layer followed by ReLU activation, the output dimension of the linear layer is also $150$. 


\paragraph{Sample 3-D Representation} We sample points on a $40 \times 40 \times 40$ grid from an area of $2.5 \text{cm} \times 2.5 cm \times 2.5 cm $ at the center of the table for FluidPour and FluidCubeShake, and on a $70 \times 70 \times 70$ grid from an area of $6 \text{cm} \times 6 cm \times 6 cm $ for GranularPush. We evaluate and include points with a density (measured by the occupancy in the predicted neural radiance fields) larger than $0.99$. Then we subsample the inferred points with FPS with a ratio of around $5\%$ for FluidPour and $10\%$ for FluidCubeShake and GranularPush.


\paragraph{Build Graph} To build graph based on the sub-sampled point-cloud, we set the neighbour distance threshold to be $0.2, 0.15, 0.15$ for FluidPour, FluidCubeShake and GranularPush respectively.


\section{Training Details}


%To train the visual head, we use a learning rate of $1e^{-4}$ with the Adam optimizer. 
%ReduceOnPlateau as the learning rate scheduler.

We sample $64$ points through each ray in the scene to compute the rendering loss when we are training our visual-head. To do paralleling sample from rays, we set the chunk size of NeRF query function $f$ to be $1024*64$.
This can be trained on one RTX-3090 within five hours to get a good visual head perception module that can be used for the following work of point-cloud sampling.


To train our dynamics head, we set batch size to $4$ for all three environments. The learning rate is set to be $1e^{-4}$, using Adam as optimizer. We train the model for $20, 30, 40$ epochs for FluidPour, FluidCubeShake and GranularPush respectively. It takes about $10\sim 15$ hours  to train the dynamics model on one single RTX-3090 for all the three environments.

\section{Dataset Samples}\label{appendix-dataset}

In this section we will give more detailed demonstration of our datasets. Our datasets are generated by NVIDIA Flex in simulation environment, where we can build and scene, add objects and make them move, the relatively accurate physics engine helps us get the movement of points in the scene.  Our dataset focuses on fluid environment, include water, granular and water+cube.

We simulate three kinds of trajectories to represent three basic movement in our daily life: Pour, Shake and Push. Each of the three types (Pour, Shake and Push) has 500 videos of trajectories taken from 6 views, each trajectory has 300 frames.
For each of the three types of video (500 videos), they can be divided into five different settings to make the dataset more diverse. Among these five different settings, the first four of them are regarded as \textbf{interpolate} setting and the last setting is viewed as \textbf{extrapolate} setting. The detailed settings can be referred to in  Table \ref{settings}. Samples from three different kind of envrionments are shown in Figure \ref{pour_sample}, \ref{shake_sample} and \ref{push_sample}. For training-testing separation, we use the separation ratio to be $0.8$, it should be noted that all trajectories for the extrapolate settings are used for testing and will not show up during the training process.

\begin{figure}
    \centering
    \includegraphics[scale=0.4]{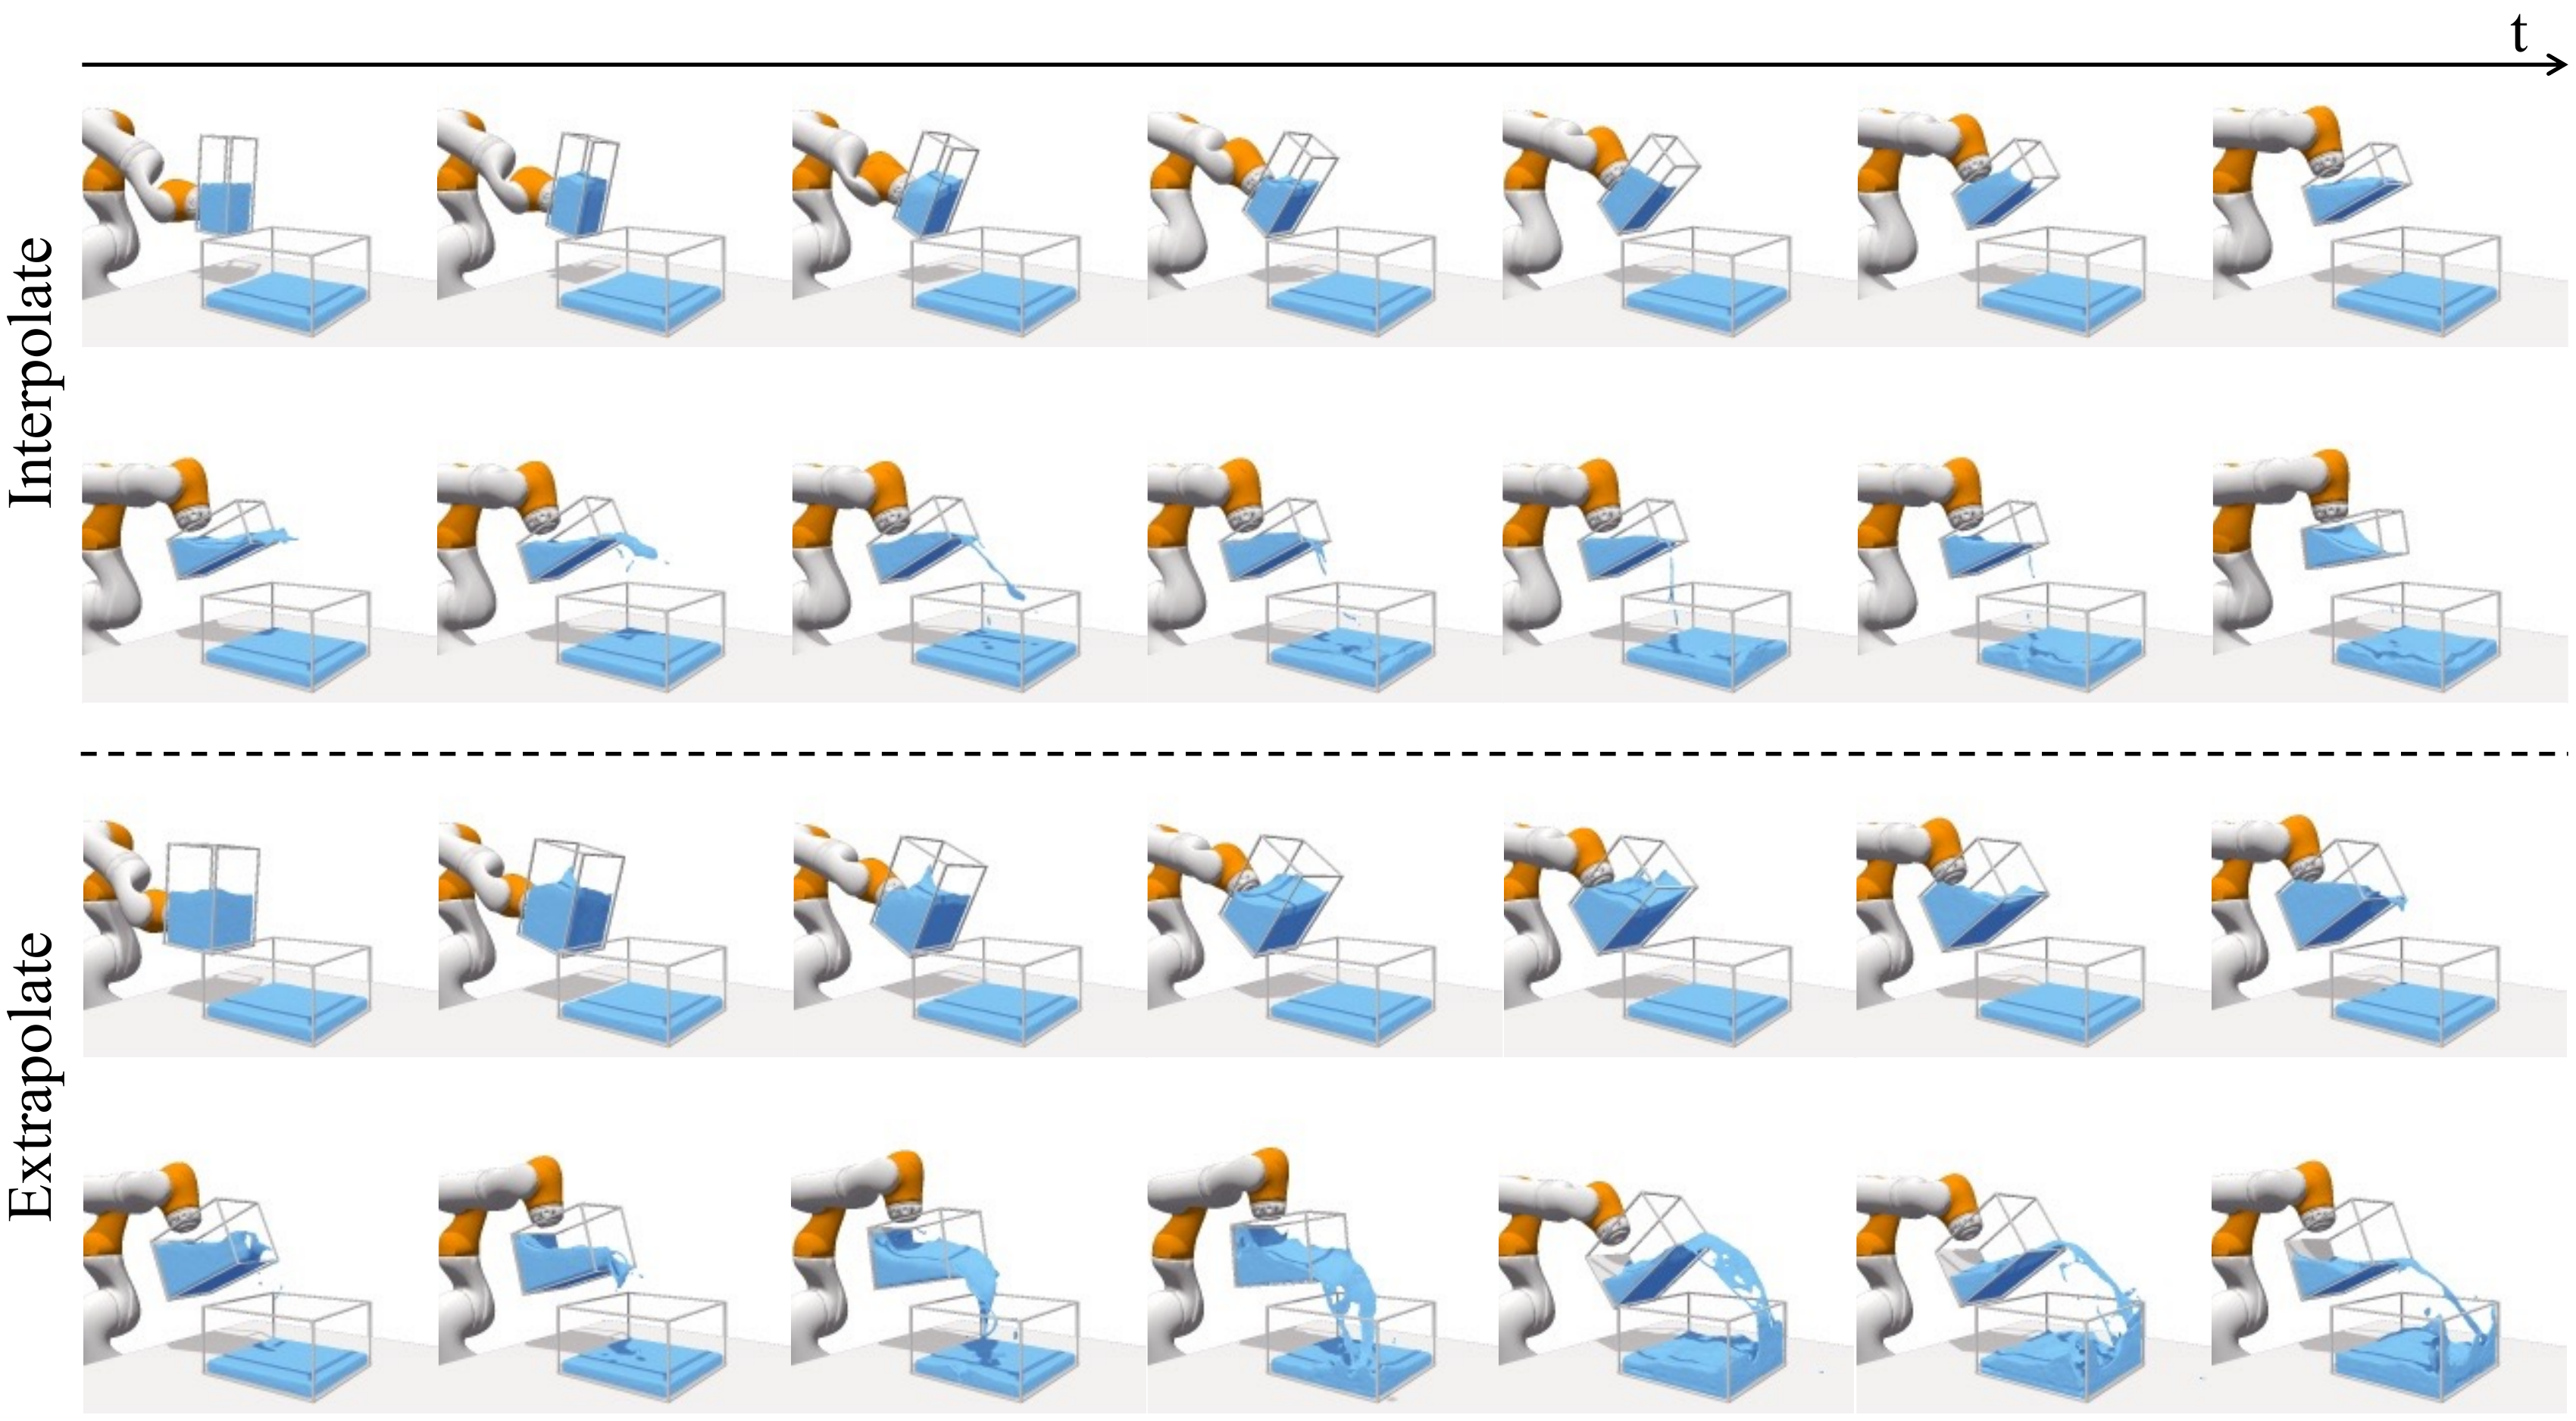}
    \caption{Caption}
    \caption{Sample of FluidPour Dataset: the sampling interval is 20 frames, the frames above the blue line are for \textbf{interpolate} data and the other part is for \textbf{extrapolate} data.}
    \label{pour_sample}
\end{figure}

\begin{figure}
    \centering
    \includegraphics[scale=0.4]{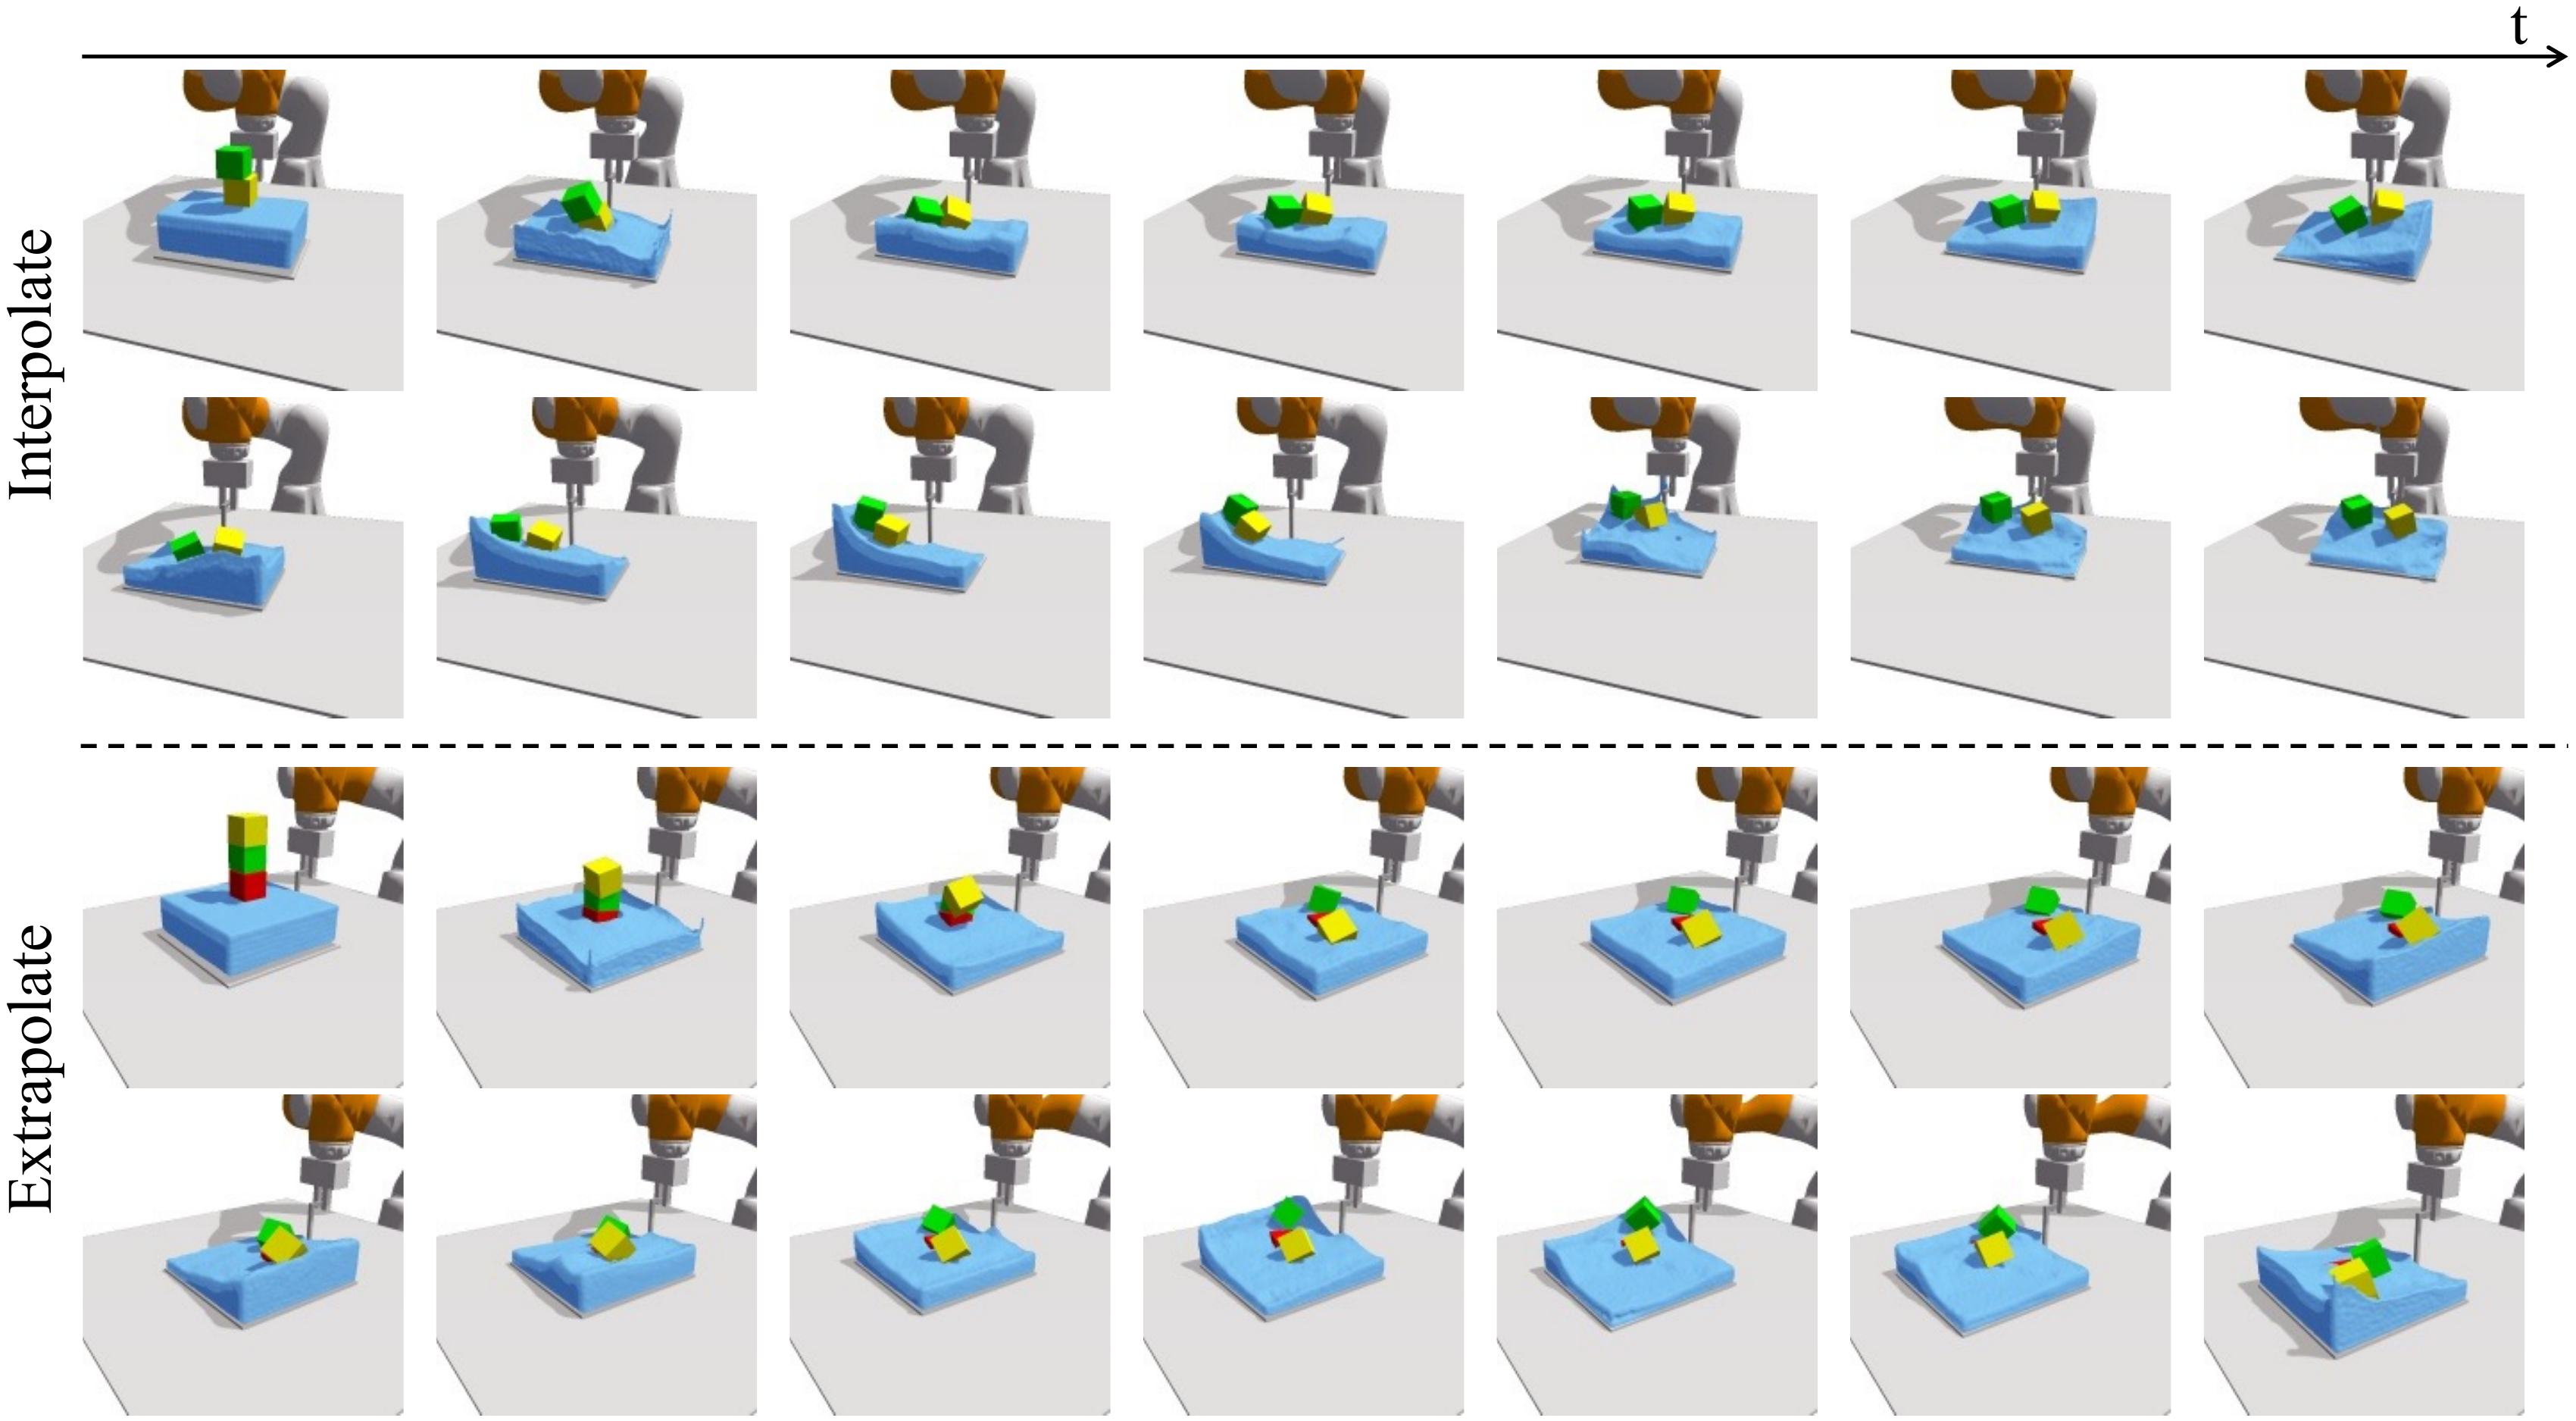}
    \caption{Sample of FluidCubeShake Dataset: the sampling interval is 20 frames, the frames above the blue line are for \textbf{interpolate} data and the other part is for \textbf{extrapolate} data.}
\label{shake_sample}
\end{figure}

\begin{figure}
    \centering
    \includegraphics[scale=0.4]{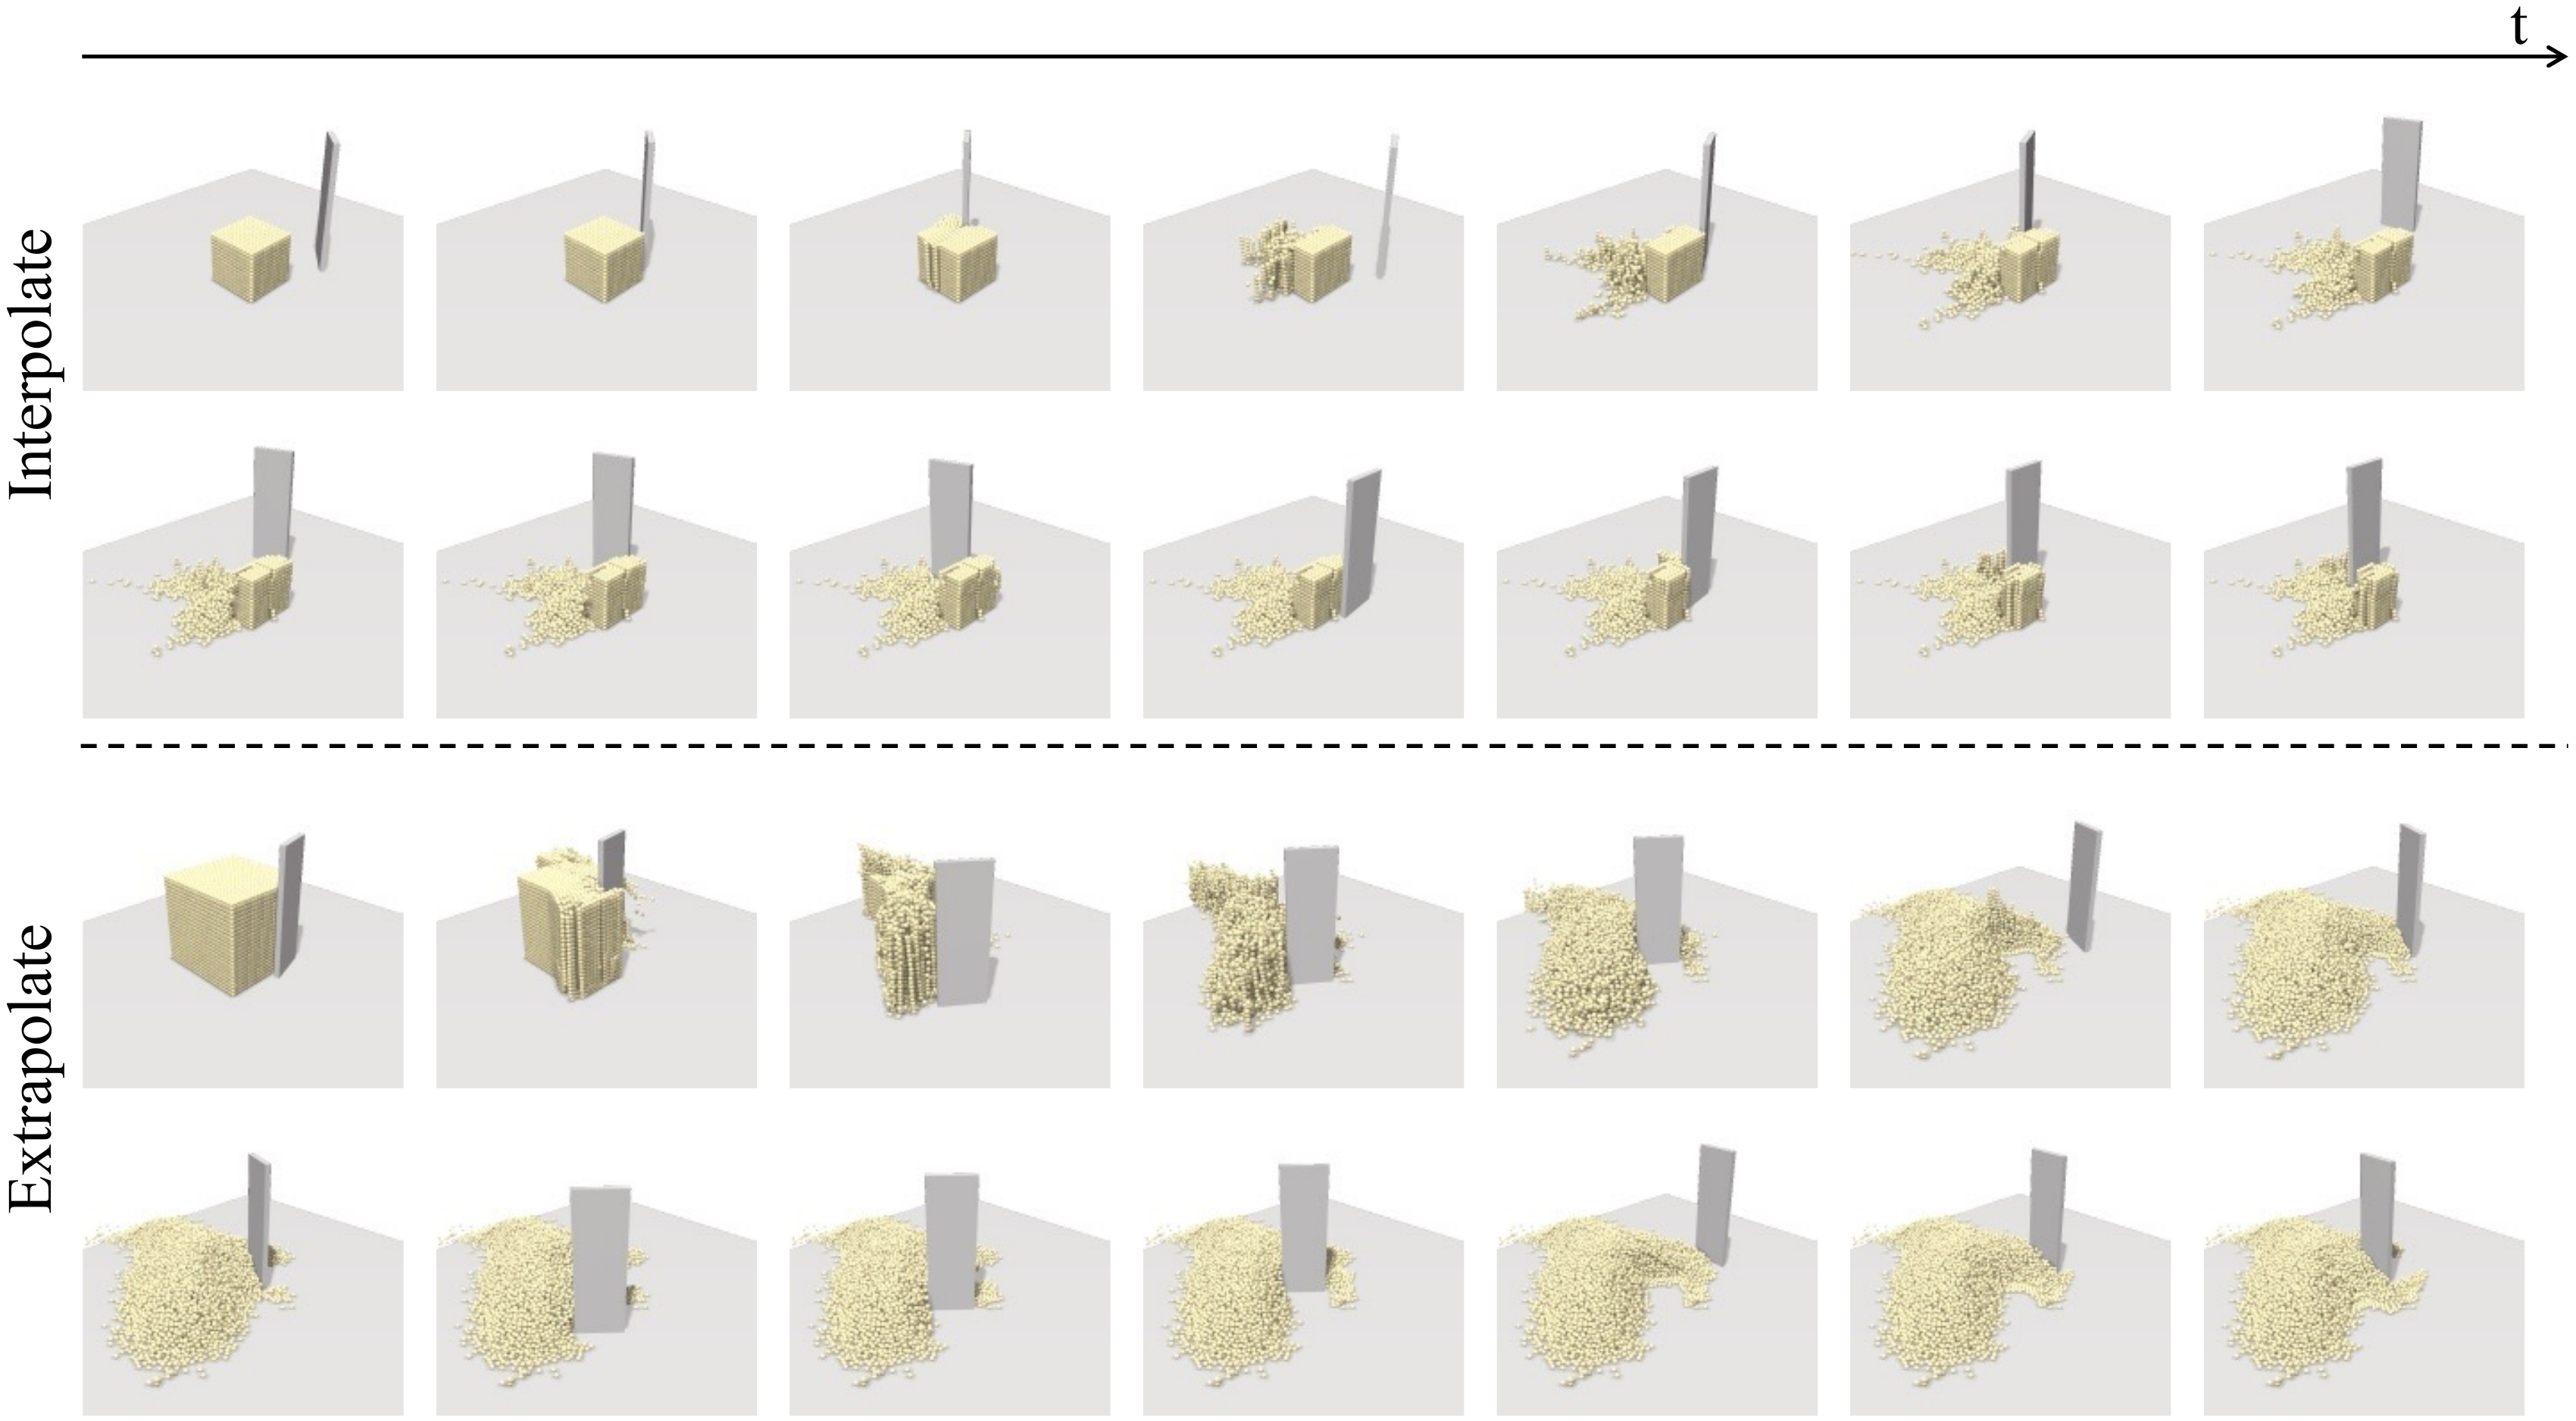}
    \caption{Sample of GranularPush Dataset: the sampling interval is 20 frames, the frames above the blue line are for \textbf{interpolate} data and the other part is for \textbf{extrapolate} data.}
\label{push_sample}
\end{figure}


\begin{figure}
    \centering
    \includegraphics[scale=0.4]{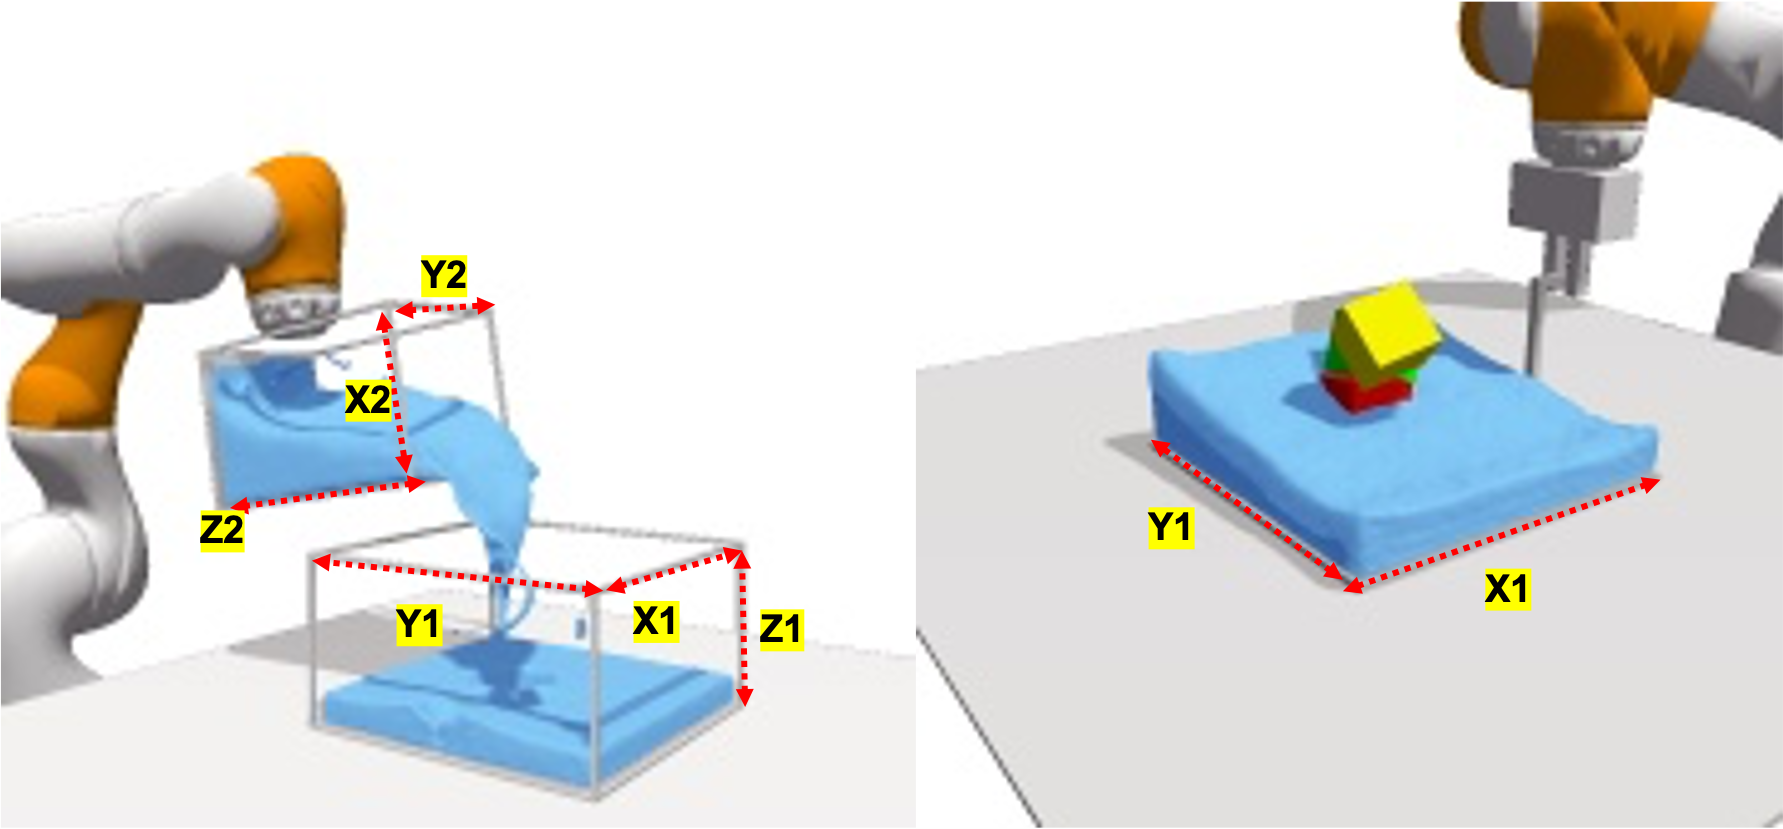}
    \caption{Labels of container shape referred to in Table \ref{settings}}
    \label{container_shape}
\end{figure}

\begin{table}[]
    \centering
    \begin{tabular}{c|c|c|c|c|c|c}
     \hline
    SceneName & Params &   Env1 &  Env2 & Env3 & Env4 & Extrapolate \\
     \hline
     \multirow{7}*{Pour} & X1    & 0  &  0 & 0  & 0 & 0 \\
                         & Y1  & 0  &  0 & 0  & 0  & 0  \\
                         & Z1     & 0  &  0 & 0  & 0  & 0  \\ 
                        & X2     & 0  &  0 & 0  & 0  & 0  \\ 
                        &  Y2      & 0  &  0 & 0  & 0  & 0  \\ 
                        &  Z2      & 0  &  0 & 0  & 0 & 0 \\ 
                        & AmountofWater    & 5125  &  5125 & 6125  & 5375 & 7625 \\
      \hline
      \multirow{4}*{Shake} & X1     & 0  &  0 & 0  & 0  & 0  \\ 
                        &  Y1      & 0  &  0 & 0  & 0  & 0  \\ 
                        &  CubeNumber  & 1  &  1 & 2  & 2 & 3  \\
                        & Water   & 2173  &  3322 & 3322  & 4858 & 4983 \\
      \hline
      \multirow{1}*{Push} & GranularNumber  & 2197  &  4032 & 5832  & 9261 & 12167 \\
                        
      \hline
    \end{tabular}
    \caption{Environment Settings: settings include some basic components of the scene, e.g. shape of container, amount of water, number of cubes. Labels can be referred to in Figure \ref{container_shape}}
    \label{settings}
\end{table}

\begin{figure}
    \centering
    \includegraphics[scale=0.4]{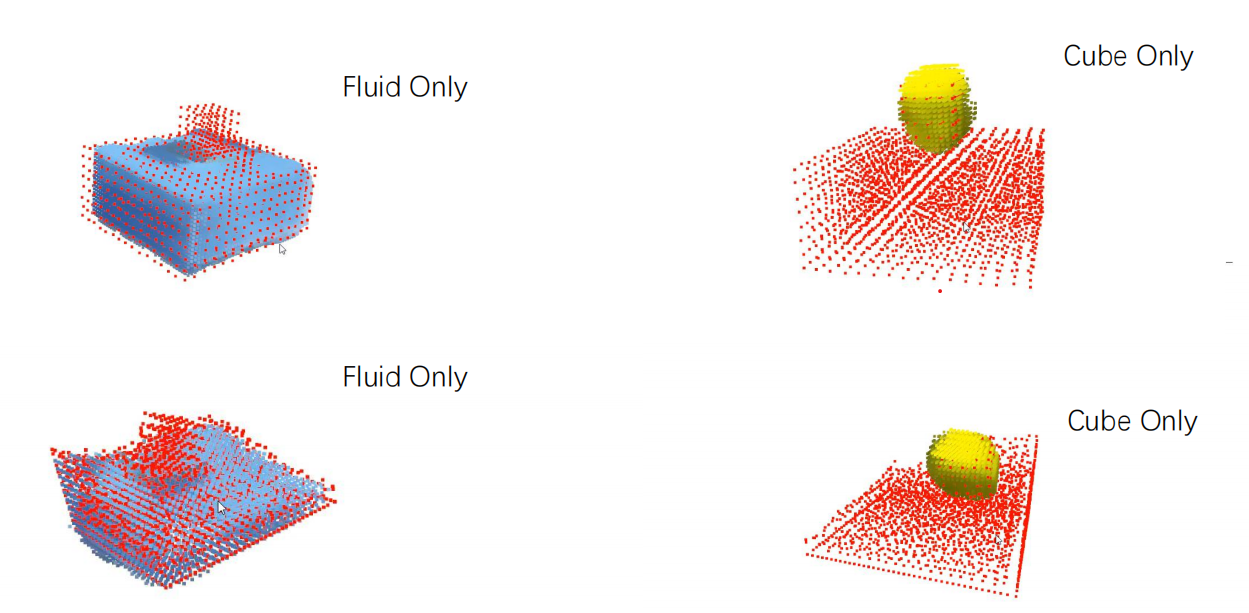}
    \caption{Example: instance segmentation through color in visual head 3d-pointcloud, red points are ground truth positions}
    \label{fig:my_label}
\end{figure}





\section{More  Qualitative  Results for Visual Head Reconstruction}


\section{More Qualitative Results for Dynamics Prediction}





\section{Potential Society Impact}
\modelname~can be applied to a wide range of down-stream applications, including general scene understanding tasks, robotics manipulation, 3D generative models, and differentiable physics engines. Out work shows the possibility of learning dynamics models from raw sensory inputs, opening up the opportunity to automate the design of differentiable physics engine though data-driven learning algorithms. Predictions from our model is highly interpretable which makes it straightforward to explain model behaviors and re-purpose the outputs for downstream applications. Though data-driven approaches are potentially more scalable, it also brings in the concern that it might be hard to ensure the model behavior to be robust under sensor noise and adversarial attacks, and to fully mitigate data biases. Bringing in advanced technique from ML robustness will be one critical future avenue to pursue.


\subsection{3D point representation from trained perception module}

\begin{figure}[h!]
    \centering
    \includegraphics[width=.8\linewidth]{imgs/appendix/seg.png}
    \caption{
    \textbf{Qualitative Reconstruction and Segmentation Results of the Perception Module.} We show on the left reconstructed 3D shape of the fluid and on the right reconstructed 3D shape of a cube floating in the fluid. Red points are ground truth point positions.}
    \label{fig:my_label}
\end{figure}
% Figure-6 : 
